# Supplementary material for: Asynchronous I/O -- With Great Power Comes Great Responsibility
Source: arXiv:2411.16254 source file (2024-11-25)
Supplement: Supplementary file 1 [file appendix.tex]

\appendix

\section{Research Methods}
\label{sec:appendix_methods}

% if we actually end up including some benchmarks and have space for them.... then put setup and bench methods etc here....
